# Supplementary material for: RotLSTM: Rotating Memories in Recurrent Neural Networks
Source: arXiv:2105.00357 source file (2021-05-01)
Supplement: Supplementary file 1 [file appendix.tex]

\section{bAbI tasks}

A summary of all bAbI tasks is shown in Table~\ref{table:babi} for reference.

% Please add the following required packages to your document preamble:
% \usepackage{booktabs}
% \usepackage{graphicx}
\begin{table}[bh]
\centering
\caption{Descriptions of bAbI dataset tasks.}
\label{table:babi}
\resizebox{\textwidth}{!}{%
\begin{tabular}{@{}rlrl@{}}
\multicolumn{1}{l}{\#} & Description                                  & \multicolumn{1}{l}{\#} & Description                        \\ \midrule
\textbf{1}             & Factoid QA with one supporting fact & \textbf{11}            & Basic coreference                  \\
\textbf{2}             & Factoid QA with two supporting facts         & \textbf{12}            & Conjunction                        \\
\textbf{3}             & Factoid QA with three supporting facts       & \textbf{13}            & Compound coreference               \\
\textbf{4}             & Two argument relations: subject vs. object   & \textbf{14}            & Time manipulation                  \\
\textbf{5}             & Three argument relations                     & \textbf{15}            & Basic deduction                    \\
\textbf{6}             & Yes/No questions                             & \textbf{16}            & Basic induction                    \\
\textbf{7}             & Counting                                     & \textbf{17}            & Positional reasoning               \\
\textbf{8}             & Lists/Sets                                   & \textbf{18}            & Reasoning about size               \\
\textbf{9}             & Simple Negation                              & \textbf{19}            & Path finding                       \\
\textbf{10}            & Indefinite Knowledge                         & \textbf{20}            & Reasoning about agent's motivation \\ \bottomrule
\end{tabular}%
}
\end{table}
