# Supplementary material for: RotLSTM: Rotating Memories in Recurrent Neural Networks
Source: arXiv:2105.00357 source file (2021-05-01)
Supplement: Supplementary file 2 [file appendix_gru.tex]

\section{RotGRU}

Unlike the LSTM, the \ac{GRU} unit only has a cell state that can be interpreted as output when needed. Intuitively we want the transformation matrix to enable the unit to learn more compact, richer representations. The rotation is inserted at the \emph{remember} ($\mathbf{r}$) gate to avoid applying a transformation on the outputs. Figure~\ref{fig:RotGRU} illustrates a RotGRU unit.

The RotGRU equations are the following:
\begin{align}
	\mathbf{x} &= [\mathbf{h_{t-1}},  \mathbf{x_t}], \\
	\mathbf{z_t} &= \sigma(\bm{W}_{\text{z}} \mathbf{x} + \mathbf{b}_\text{z}), \\
	\mathbf{d_t} &= \mathbf{h_{t-1}} \circ \sigma(\bm{W}_{\text{r}} \mathbf{x} + \mathbf{b}_\text{r}), \\
	\bm{U} &= f(\bm{W}_{\text{rot}} \mathbf{x} + \mathbf{b}_\text{rot}), \\
	\mathbf{r_t} &= \bm{U}\mathbf{d_t} \\
	\mathbf{\hat{h}_t} &= \tanh(\bm{W}_\text{h}[\mathbf{r_t}, \mathbf{x_t}] + \mathbf{b}_\text{h}), \\
	\mathbf{\mathbf{h}_t} &= (1-\mathbf{z_t}) \circ \mathbf{h_{t-1}} + \mathbf{z_t} \circ \mathbf{\hat{h}_t}.
\end{align}

\begin{figure}[h]
\begin{center}
\includegraphics[width=\linewidth]{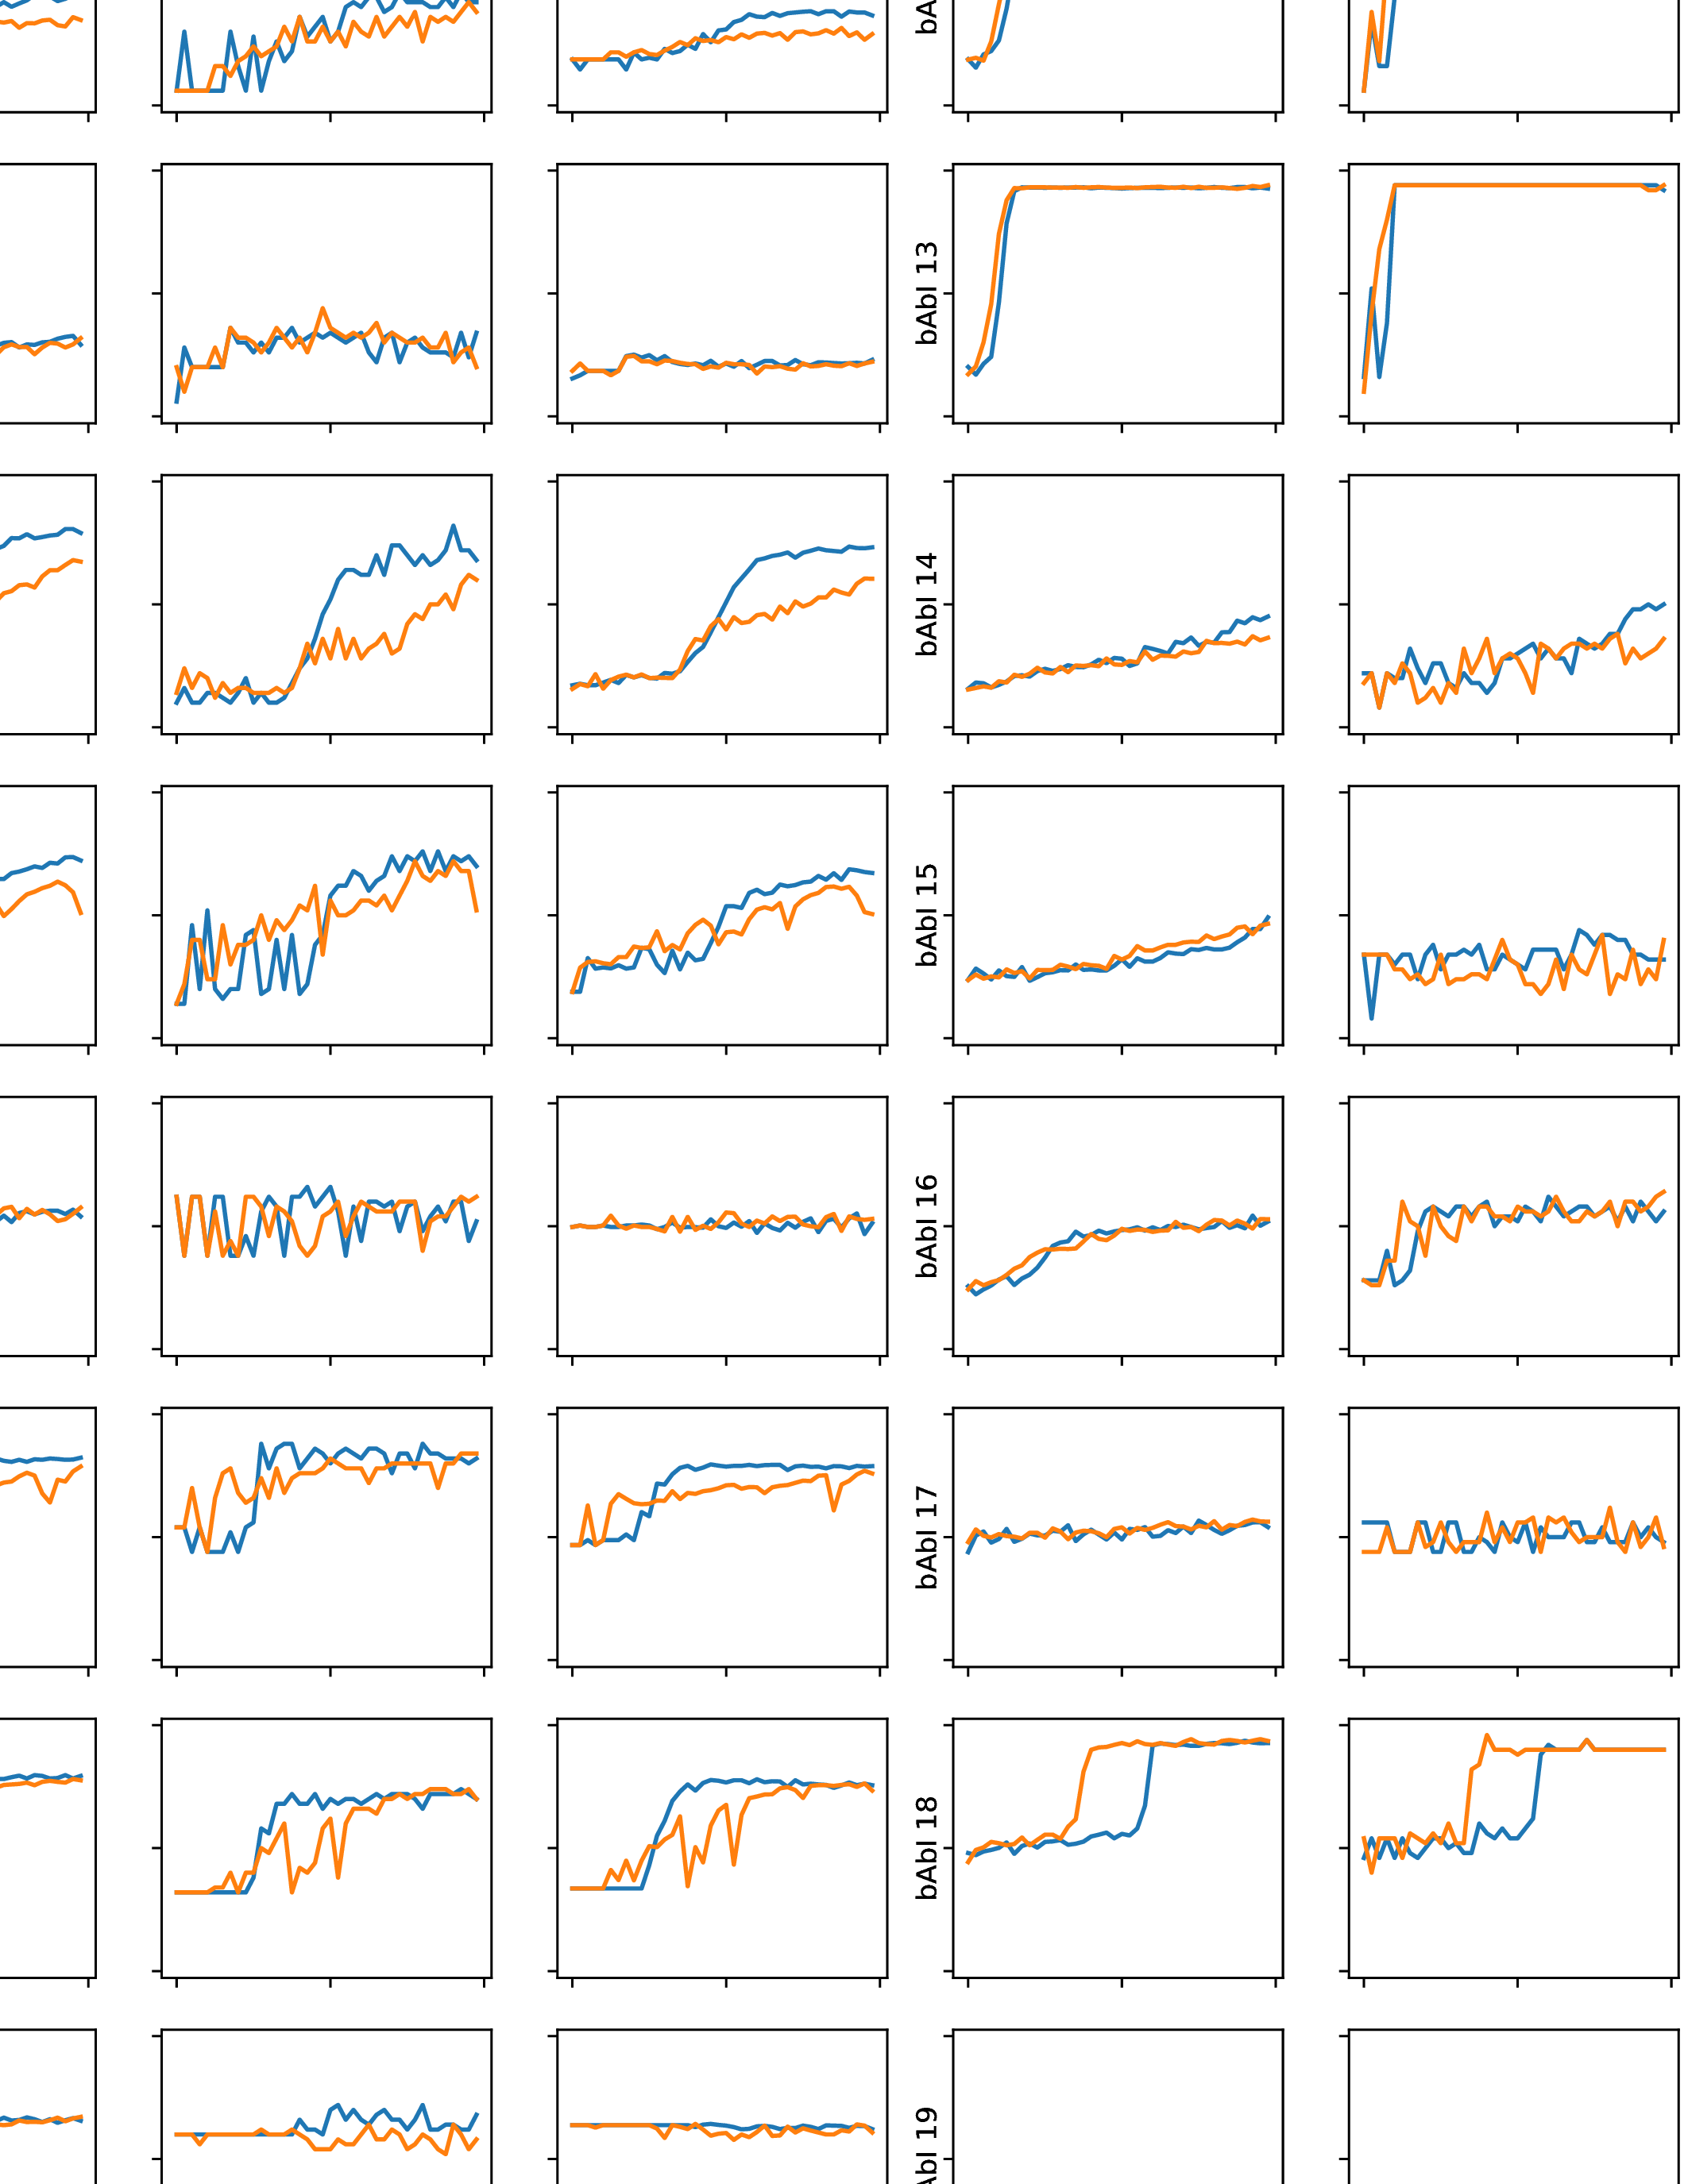}
\end{center}
\caption{Accuracy comparison on training, validation (val) and test sets over 40 epochs for GRU and RotGRU models. The models were trained 5 times and shown is the average accuracy and in faded colour is the standard deviation. Test set accuracy was computed every 10 epochs.}
\label{fig:gru_converge}
\end{figure}

\begin{figure}[h]
\begin{center}
\includegraphics[width=0.8\linewidth]{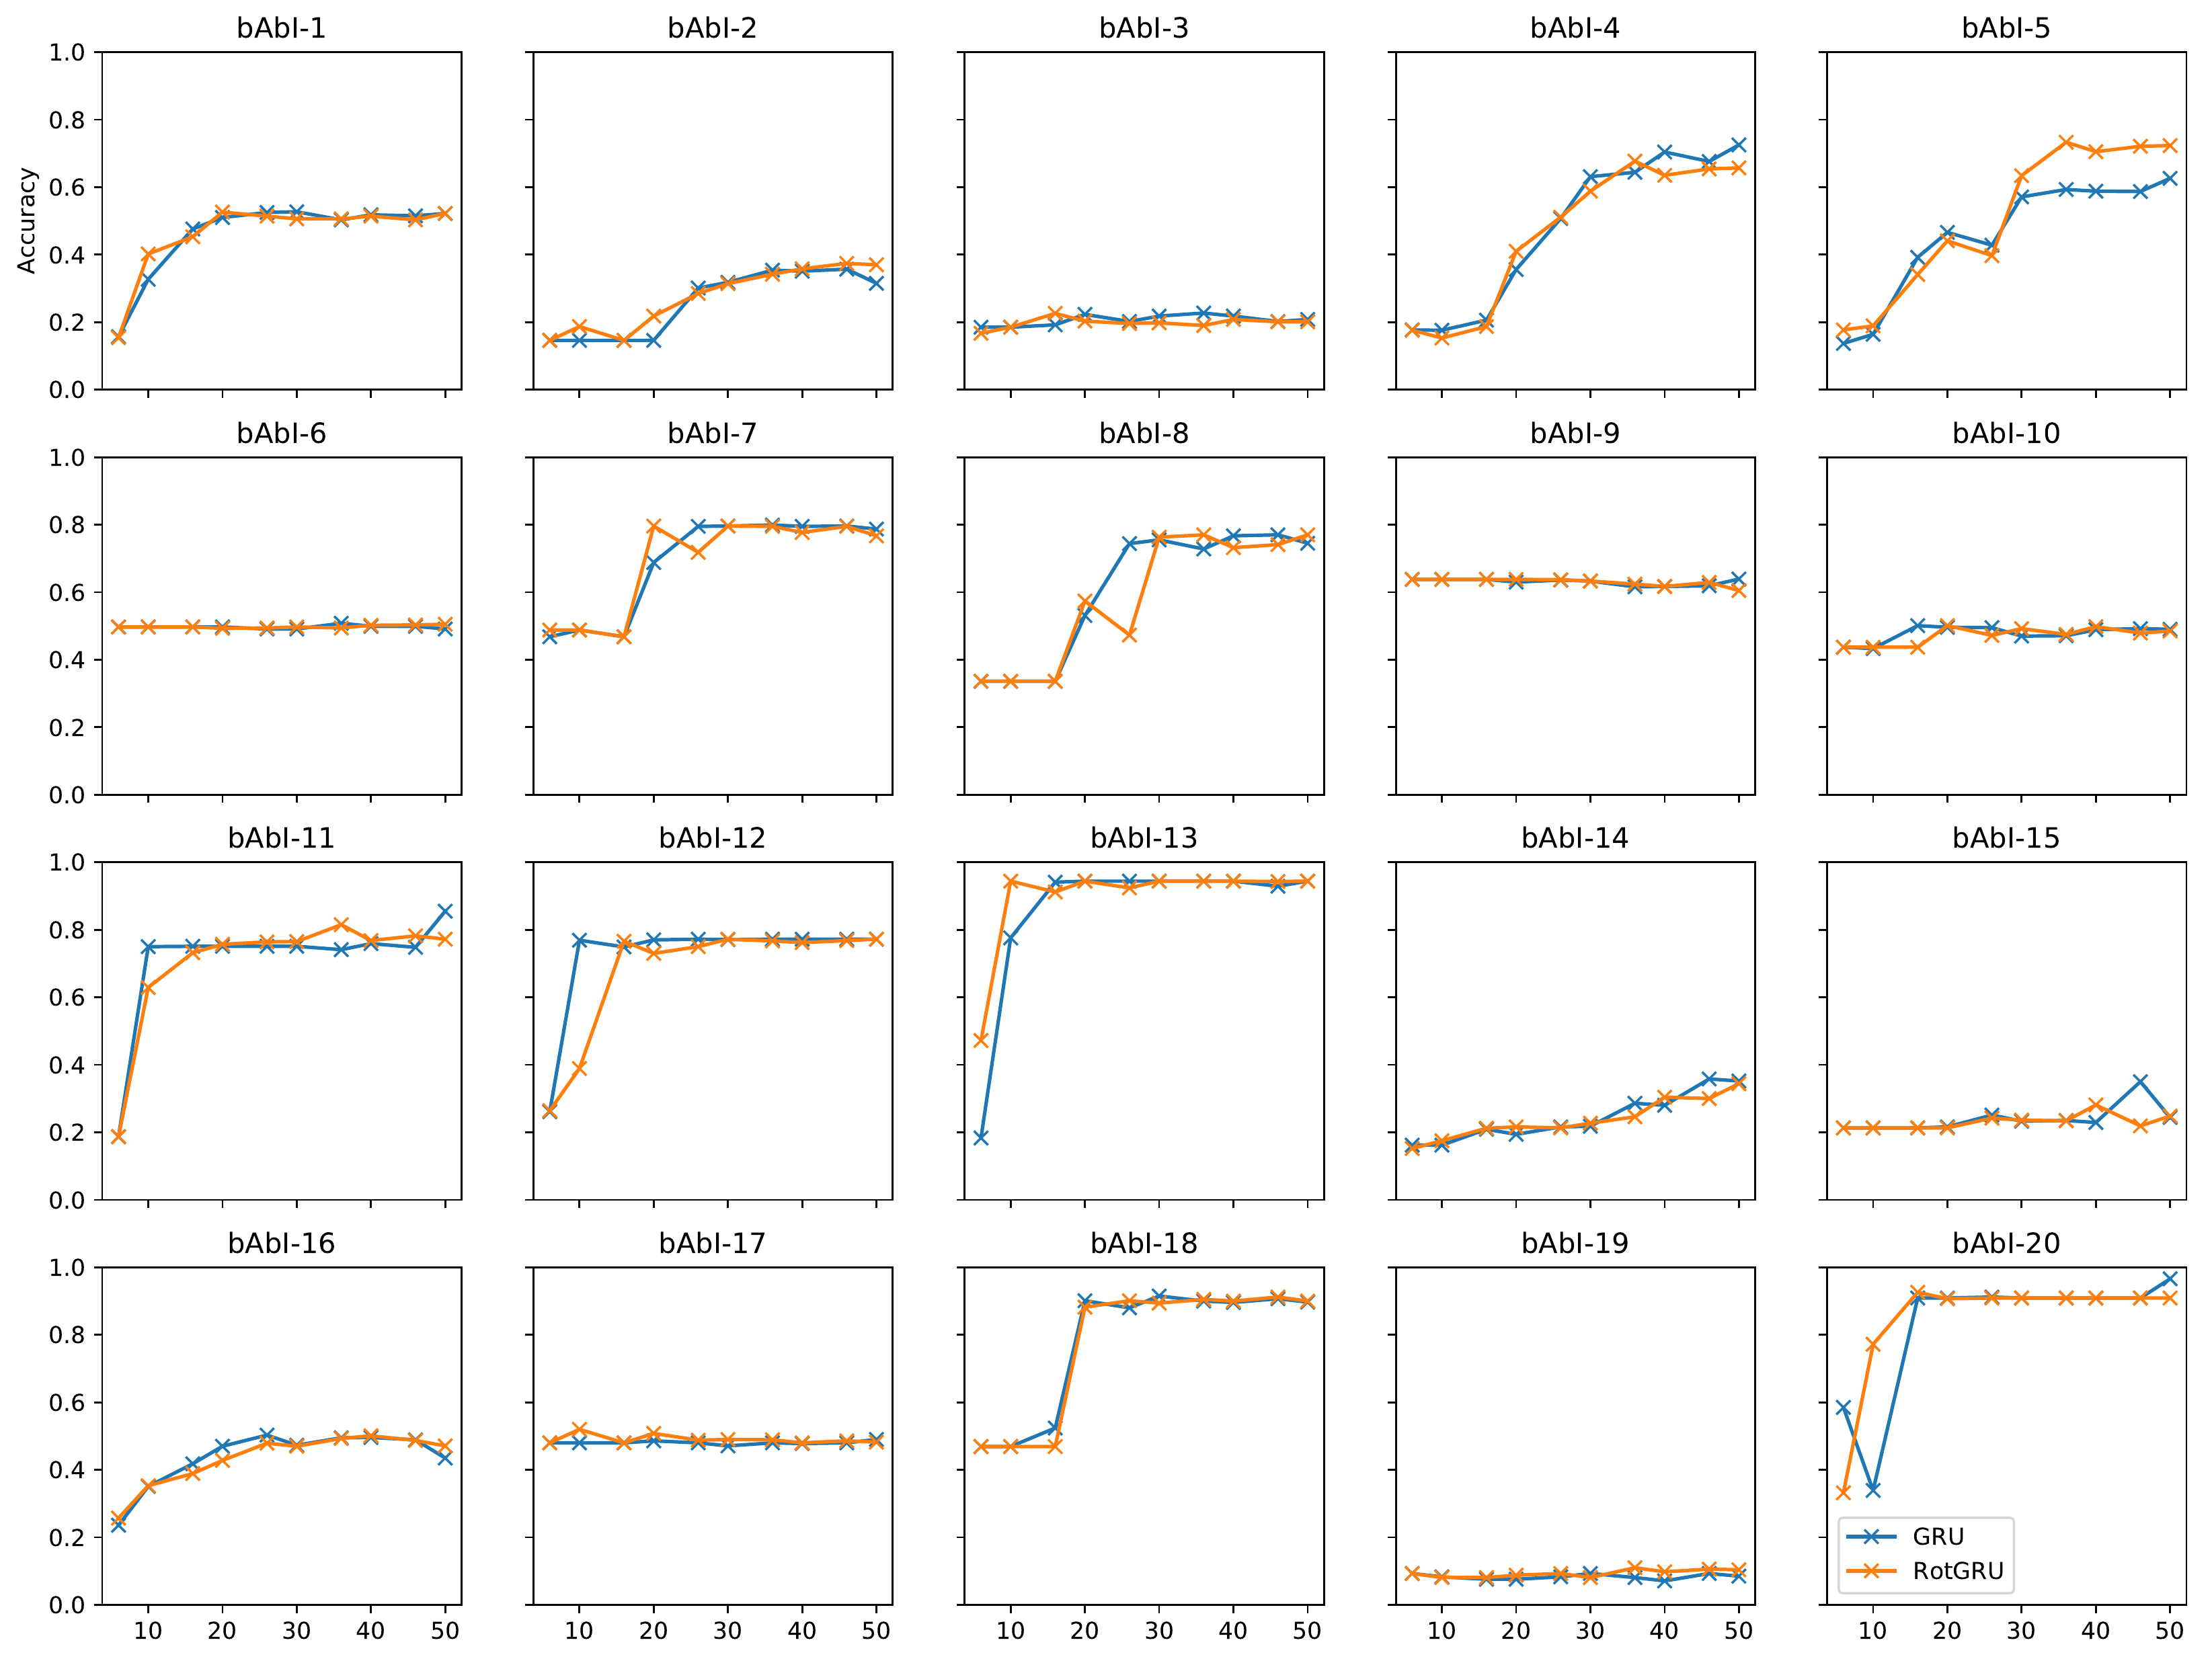}
\end{center}
\caption{Accuracy on the test set for the GRU and RotGRU while varying the cell state size.}
\label{fig:state-size-fig-gru}
\end{figure}

 The GRU based models do not show the same improvement and our tests show mostly no change in performance whether we use rotations or not.
 \subsubsection{GRU and RotGRU}

 The same does not hold for the GRU cell, which performs better without rotation capabilities. Future work will qualitatively explore why this is the case and whether hidden state transformations can improve GRU performance.
